# Supplementary material for: Fast, multicolour optical sectioning over extended fields of view by combining interferometric SIM with machine learning
Source: arXiv:2311.00089 source file (2023-10-31)
Supplement: Supplementary file 1 [file OS_SIM_Paper_Supplementary_Material__BioArXiv_format.pdf]

# Fast, multicolour optical sectioning over extended fields of view by combining interferometric SIM with machine learning: Supplementary Material

## 1 Comparison of photobleaching behaviour between point scanning confocal microscopy and ML-OS-SIM

An advantage of machine-learning optical sectioning structured illumination microscopy (ML-OS-SIM) over the widely used point scanning confocal technique is that imaging can be performed more quickly and at lower illumination intensities, resulting in less photodamage to the sample. To quantify this, two volumes of the same fixed Vero cell sample were imaged with similar imaging parameters and the reduction in the image brightness over time measured. Illumination intensity was chosen to achieve similar image quality, as judged visually. Other parameters were kept the same, as outlined in Table 1. Results are shown in Fig. 1.

Table 1: **Table of imaging parameters for comparing ML-OS-SIM and confocal microscopy**

| Parameter | Value |
|---|---|
| Objective lens | UPLSAPO60XW, Olympus |
| Field of view | $44 \times 44\,\mu m^2$ |
| Pixels | $512 \times 512$ |
| Volume (X × Y × Z) | $44 \times 44 \times 10\,\mu m^3$ |
| Z sampling | $0.5\,\mu m$ |
| Pixel size | 86 nm |

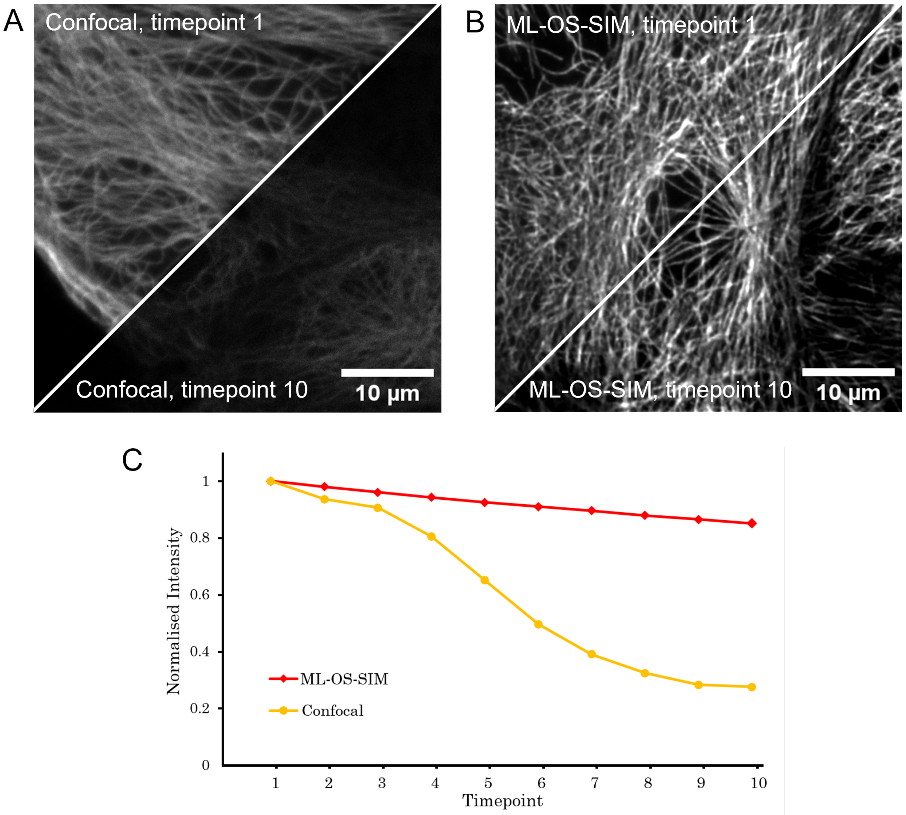


Figure 1: Machine-learning optical sectioning structured illumination microscopy (ML-OS-SIM) reduces photobleaching compared to confocal microscopy. A) 3D projections of the first and tenth timepoints when imaging a $44\,\mu m \times 44\,\mu m \times 10\,\mu m$ volume using confocal microscopy. Images show significant bleaching over time. B) Reconstructed 3D projections of the first and tenth timepoints when imaging the same size volume using ML-OS-SIM. The brightnesses of the images are proportional to the brightness of the raw data, and show minimal bleaching over time. C) The normalised brightness of the images as a function of the timepoint or number of volumes imaged. Confocal shows significantly faster bleaching owing to the higher laser power and longer imaging time required. A comparison of subfigures A and B shows that similar imaging performance was obtained using the imaging parameters set for the two methods. Images are of immunostained $\beta$-tubulin in fixed Vero cells, illuminated with $\lambda = 561\,\text{nm}$ light. Scale bars $= 10\,\mu m$.

## 2 Optical layout

A diagram of the optical layout for interferometric SIM pattern generation is shown in Fig. 2.

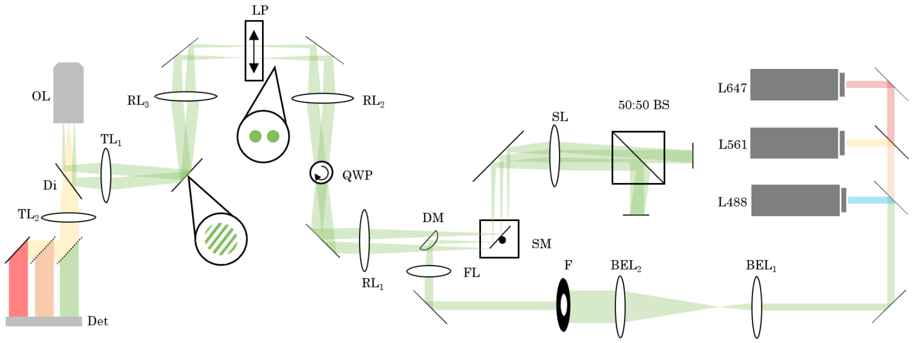


Figure 2: Optical layout for interferometric SIM pattern generation. Three laser lines (**L**) with wavelengths 491 nm (Cobolt Calypso, 200 mW), 561 nm (Oxxius SLIM-561-150, 500 mW) and 647 nm (Toptica iBeam SMART, 100 mW) are combined coaxially and the beam is then expanded and collimated by two lenses ($\mathbf{BEL}_{1,2}$) to flatten the intensity across the field of view. A field stop (**F**) restricts the excited area of the sample to minimise unwanted photodamage. The excitation beam is focused by a focusing lens (**FL**, Thorlabs, AC254-150-A) and reflected by a D-shaped mirror (**DM**, Thorlabs, PFD10-03-F01) onto a galvanometric scan mirror (**SM**, Scanlab, dynAXIS-M) which directs the beam through a scan lens (**SL**, Thorlabs, AC508-150-A) and into the Michelson interferometer. The interferometer comprises a 2-inch 50:50 beam splitter cube (**BS**, Thorlabs, BS031) and a pair of $\frac{1}{2}$-inch mirrors (Thorlabs, BB05-E01) mounted on micrometer translation stages (Thorlabs, XRN25C/M). The beamlets returning from the interferometer are descanned by the scan mirror and relayed to the microscope by a series of 150 mm focal length relay lenses, $\mathbf{RL}_{1-3}$ (Thorlabs, AC508-150-A). Polarisation is controlled by a quarter wave plate (**QWP**) and linear polariser (**LP**). The two beamlets are then directed into the inverted microscope frame (Olympus, IX73) and onto the back focal plane of the objective lens (**OL**, Olympus, UPLSAPO60XW) through a tube lens ($\mathbf{TL}_1$, Thorlabs TTL200A). The beamlets are focused by the objective so that they interfere in the sample plane to form a sinusoidal illumination pattern. Fluorescence signal is isolated with a quadband dichroic mirror (**Di**, Chroma, 405/488/561/647) and focused onto the detector (**Det**, PCO, edge 4.2bi). The fluorescence signal is separated into emission bands by two long-pass dichroic mirrors enabling multiple colour channels to be imaged side-by-side on the detector.

# 3 Optical alignment methodology for ML-OS-SIM

Alignment can be optimised using a monolayer of sub-diffraction-sized fluorescent beads on a glass coverslip (Fig. 3). The two primary checks that need to be performed are the periodicity of the excitation fringes and the alignment of the beamlets at the back aperture of the objective lens.

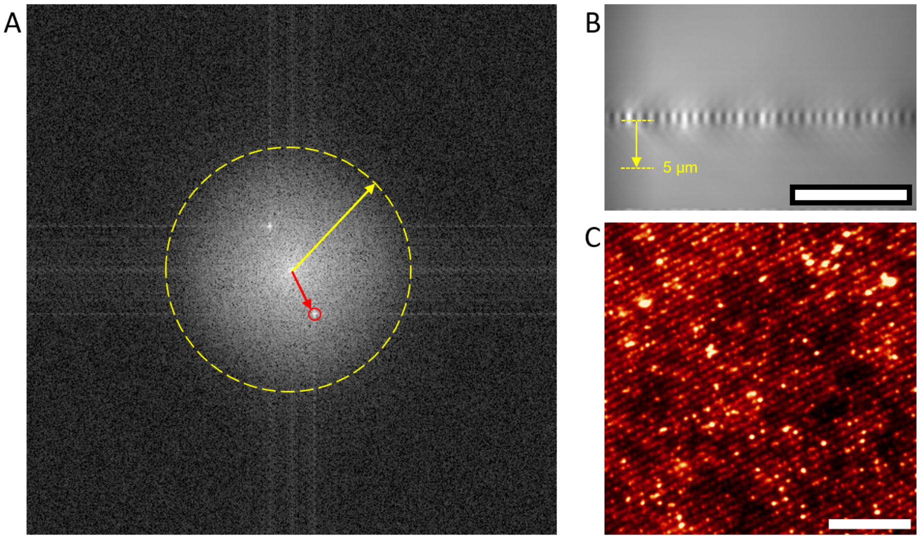


Figure 3: System alignment checks. A: The periodicity of the stripes can be optimised by visualising the Fourier transform of a raw OS-SIM frame. For best performance, the spatial frequency of the pattern must be half of the cutoff. This can be confirmed in the Fourier transform by ensuring that the distance of the peaks from the centre (red arrow) is half the radius of the supported frequency cutoff (yellow arrow). B: $x, z$ projection of a z-stack taken through a bead monolayer. Off-axis alignment of the excitation beams will result in change in pattern phase as the height of the sample is changed. In a misaligned system, this results in tilted fringes when the 3D volume is viewed in the $x, z$ direction. Scale bar $= 5\,\mu m$. Yellow dashed line indicates a $5\,\mu m$ displacement from the focal plane. C: OS-SIM stripes visualised on a fluorescent bead monolayer. Both alignment checks can be carried out on the same sample if the bead density is optimised. Sub-diffraction beads must be sufficiently sparse to enable visualisation of the optical transfer function (A) while also being sufficiently dense to visualise the fringe pattern in the $x, z$ projection. Scale bar $= 5\,\mu m$.

# 4 Machine learning reconstruction of OS-SIM data

## 4.1 Video Super-Resolution Network

To perform high-fidelity reconstructions post-acquisition, we made use of a shifted window video-transformer network. In particular we use a video super-resolution (VSR) shifted window transformer network as previously reported. This VSR network is optimised to combine information from adjacent frames in a sequence, offering improved performance on moving structures compared to other machine learning (ML) networks. To achieve this, the input OS-SIM data sequence is concatenated into a 3D volume which is then analysed using 3D self-attention windows and multi-channel attention.

## 4.2 Residual Channel Attention Network

The architecture of the lightweight convolutional neural network (CNN) was based on the residual channel attention network (RCAN) model, which comprises sequential residual groups linked by skip connections [1]. The network consisted of three groups of ten residual blocks each with 96 filters based on a $3 \times 3$ kernel. Unlike in previously reported implementations of the RCAN architecture for SIM, the initial "head" layer was adjusted to use learnable filters with a size of $7 \times 7$ as this improved performance over smaller filters.

## 4.3 Data generation

To avoid the issue of limited training data, we adopted a transfer learning approach and chose to train the network on simulated OS-SIM data. Two separate datasets were generated for the network training with each dataset tailored for each network. For the RCAN model, where reconstruction speed requires a smaller network, the in-focus plane was simulated from a library of high-resolution static images. This aligns with the primary goal of the RCAN model: to provide the user with real-time reconstructions at the expense of robustness to the artefacts associated with moving samples. For the VSR network, these static OS-SIM data were supplemented with data simulating samples with moving structures. Here, the in-focus plane was generated from three sequential frames in video sequences from BBC nature documentaries, mimicking samples that move during acquisition. For both the VSR and RCAN training datasets, the structures of the out-of-focus planes of the sample were simulated by taking static images from the DIV2K dataset [2]. From these ground-truth images, model OS-SIM data were then generated by multiplying both the in-focus and out-of-focus planes with a sinusoidal excitation pattern and subsequently blurring them by convolution with either the in-focus or out-of-focus point spread functions (PSFs). The planes were then merged using a weighted addition. Varying levels of Gaussian and Poissonian noise were added to the raw frames after combination. The parameters for generating the PSFs and the excitation

pattern were randomised, allowing the models to generalise to data collected on a range of microscopes and in varying imaging conditions.

### 4.4 Network training

Both networks were trained in *Python* using the *Pytorch* library. The networks were trained on 5000 simulated images for 200 epochs on an Nvidia RTX3070 graphics card. For the VSR network, these 5000 simulated images were composed of 2000 static targets and 3000 moving targets. The networks were trained using the Adam optimiser. For the initial 100 epochs, the mean square error (MSE) loss function was used which was changed to the L1 absolute difference loss function. These loss functions were calculated relative to the high-resolution ground truth in-focus image. For the VSR network, the second frame in the sequence was used to provide this ground truth. Under these conditions, network training took approximately 20 h for the RCAN model and 38 h for the VSR network.

The models were first validated by demonstrating their performance on simulated 3D samples consisting of a mesh of 3D filaments (Fig. 4). A complete image formation model using ideal 3D PSFs was implemented in *MATLAB*. The background rejection ability is apparent as improved contrast in the reconstructed image. The models are additionally validated by comparison of the effective optical transfer functions (Fig. 4). The models were also validated against classical reconstruction techniques.

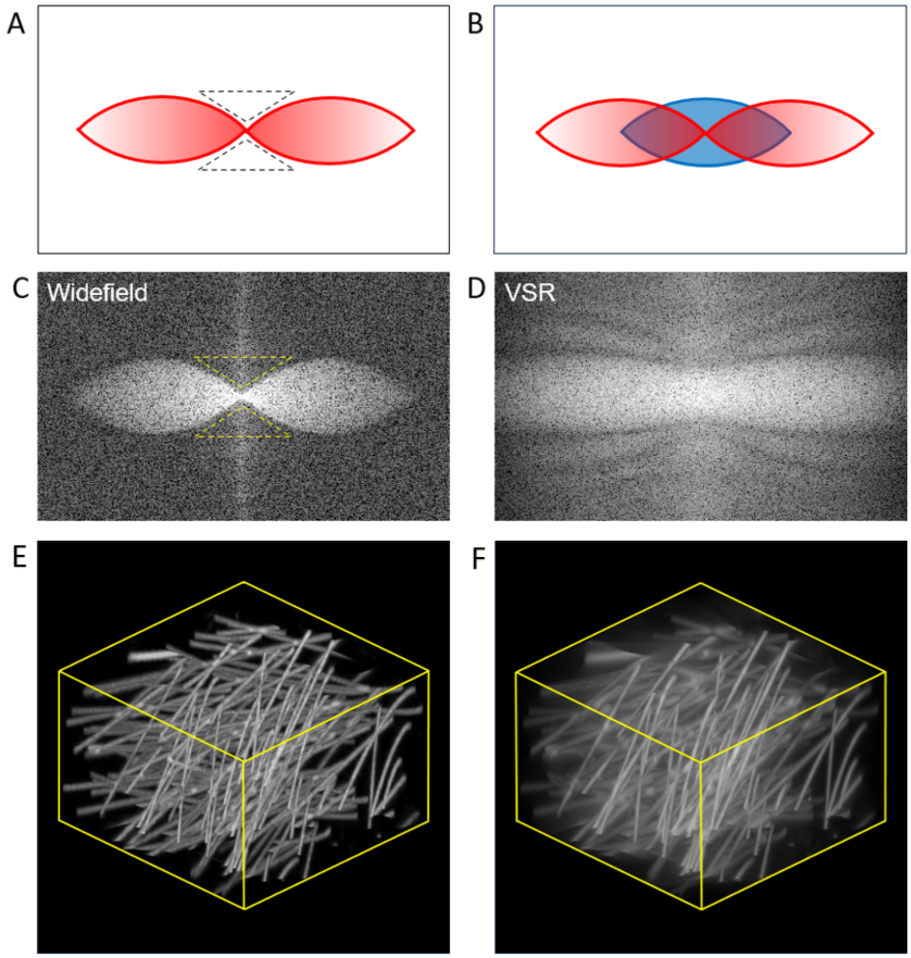


Figure 4: ML reconstruction of OS-SIM data recovers axial resolution and fills the missing cone. A: Schematic indicating the shape of the optical transfer function (OTF) of a widefield microscope in the $k_x$,$k_z$($k_y = 0$) plane. B: Ideal OTF after OS-SIM reconstruction. Upon illumination with a stripe pattern, the low spatial frequency components (blue area) can be extracted and allocated to the correct location in frequency space. C: $k_x$,$-k_z$($k_y = 0$) projection of the widefield OTF from simulated OS-SIM imaging of point sources. The bright area indicates the supported spatial frequencies. In the $k_z$ direction, a cone of frequencies (yellow dashed line) is missing. These missing frequencies contain the axial information of the sample and their absence results in the poor background rejection seen in widefield imaging. D: Calculated OTF of VSR reconstruction of simulated OS-SIM images. Compared to C, the missing cone has now been filled, indicating that axial information has been recovered in the reconstruction.

# 5 Classical reconstructions

## 5.1 Difference of squares

The basic OS-SIM images were reconstructed using the square difference (SD) approach from Neil *et al.* [3]

$$I_R^2 = (I_1 - I_2)^2 + (I_2 - I_3)^2 + (I_1 - I_3)^2 \tag{1}$$

The histograms of the raw frames $I_n$ were matched before reconstruction to compensate for variation in intensity.

## 5.2 Filtered square difference reconstruction

In addition to the classical SD approach, our ML reconstruction was tested against a corrected SD method and a filtered SD reconstruction algorithm by Li *et al.* [4] The corrected SD method compensates for uneven phase stepping of the pattern and sample drift between frames by weighting the components of the reconstruction according to the phase of the excitation pattern:

$$I_{corr.}^2 = (I_1 - I_2) + \left[ \frac{(I_2 - I_3)}{\tan\left(\frac{\phi_2 - \phi_3}{2}\right)} + \frac{(I_3 - I_1)}{\tan\left(\frac{\phi_3 - \phi_1}{2}\right)} \right]^2 \tag{2}$$

where $I_n$ are the raw images and $\phi_n$ are the corresponding relative phases of the excitation pattern, calculated using the inverse matrix approach from Cao *et al.* [5]

The mixed filtering method further refines this corrected OS-SIM image by mixing the high spatial frequency information from the widefield image with the low spatial frequency information from the OS-SIM image. The widefield image is high-pass (HP) filtered and mixed with the low-passed (LP) OS-SIM image according to a weighting parameter $\alpha$:

$$I_{filtered} = \alpha \cdot \mathbf{HP}\left(I_{widefield}\right) + (1 - \alpha) \cdot \mathbf{LP}\left(I_{corr.}\right) \tag{3}$$

This has the effect of simultaneously removing the out-of-focus light from the reconstruction while making use of the widefield image to remove the noise introduced in the SD-SIM reconstruction. The filter width is determined by the frequency of the fringe pattern and the mixing parameter is chosen based on the modulation depth of the pattern.

Both the basic and filtered SD reconstructions were calculated in *MATLAB*.

# 6 Comparison of reconstruction techniques

To quantify the improvement in reconstruction quality, simulated OS-SIM data of a filament sample were generated in *MATLAB*. Images were calculated from an artificial ground truth through multiplication with a striped excitation pattern and convolution with the PSF for a widefield microscope. The PSF was calculated using the Born and Wolf model for an emission wavelength of 600 nm using a water immersion objective lens with $NA = 1.2$ and voxels measuring $86 \times 86 \times 86$ nm. Low levels of Gaussian noise and varying levels of Poissonian noise were added to simulate imaging with a scientific complementary metal-oxide-semiconductor (CMOS) camera. Poissonian noise was simulated by sampling pixel values from a Poisson distribution scaled by $\eta \times 10^{12}$ where lower values of $\eta$ correspond to a lower number of photons emitted from the sample and correspondingly a higher noise. Figure 5 shows a comparison of the ML reconstruction methods and the filtered SD reconstruction.

The quality of the reconstructions was also tested at varying noise levels by measuring the structural similarity (SSIM) between the reconstruction and an ideal optically sectioned image (Fig. 6). This ideal image was calculated through convolution of the simulated filament sample with a model confocal PSF.

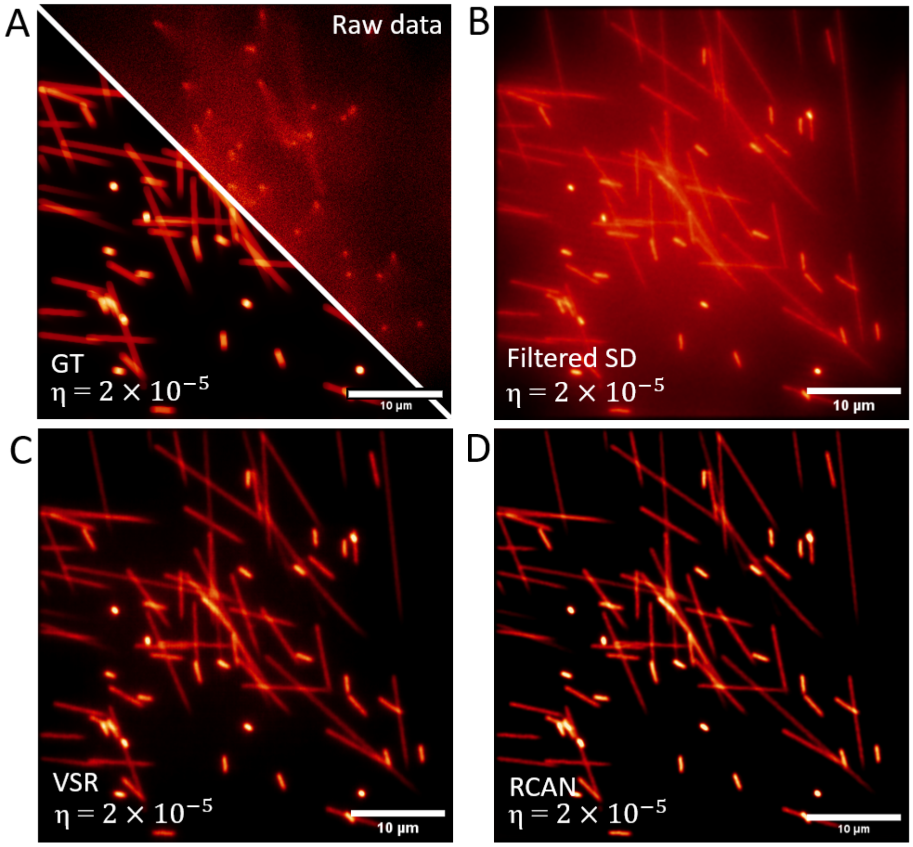


Figure 5: Machine learning reconstructions outperform square difference reconstructions at low signal-to-noise ratios. A: Comparison of the simulated ground truth (GT) confocal image and an unprocessed widefield frame. The GT image shows a mean intensity projection of 50 slices from the simulated 3D volume with no Poissonian noise added. Raw data shows the expected widefield image from a single frame, calculated as the mean of the 3 OS-SIM images acquired at that plane with a Poissonian noise factor $\eta = 2 \times 10^{-5}$. B-D: Mean intensity projections of the filtered square difference (SD), video super-resolution (VSR) and residual channel attention network (RCAN) reconstructions. Intensity projections were taken from the same 50 slices as the confocal GT and were reconstructions of simulated data with a noise level $\eta = 2 \times 10^{-5}$. Scale bars $= 10\,\mu m$, determined by the voxel size of the simulated 3D point spread function (PSF). Cubic voxels were used when calculating the 3D PSFs and each slice corresponds to a step size of 86 nm through the sample.

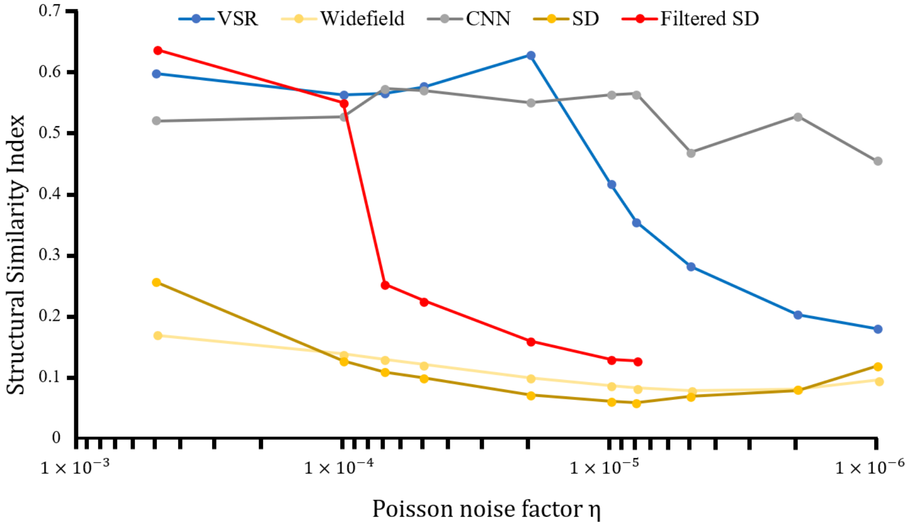


Figure 6: Error analysis of OS-SIM reconstruction methods. Measured with the structural similarity index, reconstructions with a score above 0.5 represent optically sectioned images with minimal background or artefacts (Fig. 5). All reconstruction methods show a decrease in performance as the signal level (Poisson factor, $\eta$) decreases. At the noise levels tested, filtered SD outperforms basic SD at all levels and marginally outperforms VSR and RCAN reconstructions at the lowest noise levels. As noise increases, filtered SD shows a sharp drop in performance at a noise level of $\eta = 1 \times 10^{-4}$ vs $\eta = 2 \times 10^{-5}$ for the VSR approach. On these static samples, the RCAN method continues to perform reconstructions at levels down to $\eta = 5 \times 10^{-6}$, although it is not used for post-acquisition reconstruction, as it is not optimised for the reconstruction of moving samples.

# 7 Hardware control

Image acquisition was controlled by software written in *Python*, which displayed a graphical user interface (GUI) for easy and intuitive use (Fig. 7). The software can control the camera exposure and readout, stage movement and scan mirror movement, and enables real-time viewing of reconstructed data via the GUI. Code is available in a GitHub repository [6].

The functionalities of the frames in the GUI shown in Fig. 7 are as follows. "Start/Stop Live Imaging": Simple start/stop buttons to begin and end the various processes of the system such as image acquisition, reconstruction and display. Relevant buttons in the "Saving" frame are enabled once live imaging has begun. "Saving": images can be saved in various ways using the buttons in this tab. "Start saving" will begin saving whichever image is currently being shown and continuously save images until it is pressed again. The button is relabelled "Stop saving" whilst saving is in process so this is clear to the user. In the case of 3D imaging, it will wait until the beginning of the volume to start saving, so that an integer number of stacks are recorded. "Snap shot" captures a single image and "Save stack" a single volume. In all cases, both the raw and the reconstructed images are saved in separate files, as well as a metadata file which contains relevant parameters such as which lasers are on, laser power, exposure time, time interval between captures, and, for 3D imaging, positions in z. The folder and filename to save images to can be selected by clicking the relevant buttons, which opens a dialog for straightforward selection of the directory. "Laser Control": In this frame, the lasers are turned on and off by clicking the On/Off buttons and the power can be selected using the drop-down menus. "ML Reconstruction": parameters relating to the live ML reconstruction can be entered here. These are preset at appropriate values such that clear reconstructed images should be displayed without requiring this input from the user. "Colour Channels and FOV": this frame controls which pixels in the FOV of the camera are selected as the region of interest (ROI) and subsequently processed, displayed and saved. "Imaging Parameters": values can be entered by the user to control the exposure time and, in the case of 3D imaging, the height of the volume to be imaged and the number of slices along the z direction to capture. Video parameters will control how many time points will be saved and the interval between them when saving using the "Save Video" button in the "Saving" frame. Lasers will be automatically switched off during the interval between image captures to minimise photobleaching. "Display Brightness" allows the user to increase the relative brightness of different colour channels in the display using sliders. Default setting is equal brightness. The "Imaging mode" drop-down menu can be used to select between four options: 1) display of a Fourier transform of the image, which can be used to calibrate the stripe pattern, 2) no reconstruction, which displays the raw frames captured by the camera with no processing, so that the stripe pattern illuminating the sample is visible, 3) single slice reconstruction, which displays a ML-reconstructed image of one plane in the sample and 4) volume reconstruction, which displays a maximum intensity projection of all the reconstructed slices in the range defined by

Z Min to Z Max. The "Show live images" checkbox allows the user to stop the display of images in the GUI, which can improve the image acquisition speed and reduce computational load, the "Save reconstructions" checkbox allows the user to choose whether the reconstructed images should be saved in addition to the raw data, and "Fast mode" can be selected for maximum acquisition speed without any live processing.

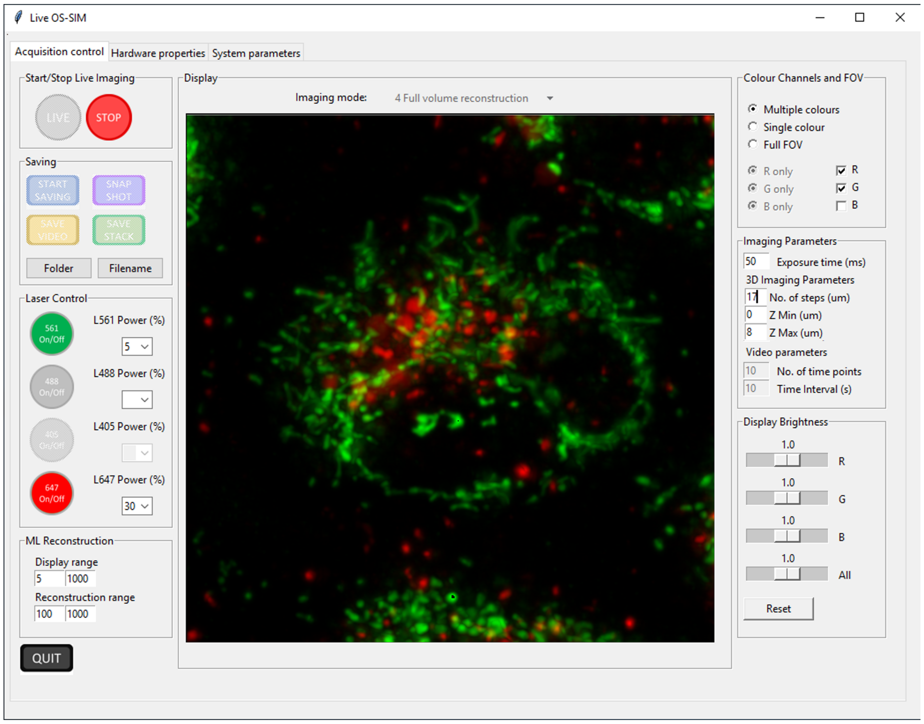


Figure 7: Graphical user interface for acquisition, real-time processing and display of OS-SIM data.

# 8 Sample Preparation

## 8.1 Bead monolayer

The monolayer was generated by air-drying 5 $\mu$L of 1:10,000 dilution of 20 nm Carboxylate-Modified Microspheres (ThermoFisher, F8786) onto a 175 $\mu$m coverglass at room temperature. Fluorescent beads were red-labelled with excitation/emission maxima 580/605 nm.

## 8.2 Live COS-7 cell culture

**Cell culture** COS-7 cells were obtained from ATCC (American Type Culture Collection, CRL-1651). These cells were grown in DMEM (Dulbecco's Modified Eagle's Medium, Sigma: D6546) supplemented with 10% heat inactivated FBS (Fetal Bovine Serum, Life Technology Invitrogen:10500064), 1% Antibiotic-Antimycotic mix (Invitrogen: 15240-062) and 2 nM Glutamax-1 (Life Technologies: 35050-038). The culture was maintained in T75 or T25 flasks at 37 °C temperature with 5% $CO_2$ atmosphere. Cells were maintained in the logarithmic phase of growth and passaged on reaching 65-75% confluence (twice weekly). For imaging, COS-7 cells were seeded into a Nunc Lab-Tek II chambered cover glass (Thermo Fisher Scientific, 12-565-335) and allowed to grow until 70% confluency.

**Transfection & labelling** COS-7 cells were transfected with 200 ng mCherry-PH plasmid (Addgene, 36075), using Lipofectamine 2000 transfection method as directed in the manufacturer's protocol. Cells were allowed to grow for a further 24 h before being subjected to imaging, to achieve optimum expression of PH domain of PLCdelta1. For labelling mitochondria, 100 nM of Mitotracker dye was added into the well from the stock of 100 $\mu$M solution and cells were incubated with the dye for 1 h before imaging. Imaging was performed with a stage-top incubator (OKOLab) at 37°C and 5% $CO_2$.

## 8.3 Fixed Vero cell culture

Vero cells (from monkey kidney tissue) were plated into 8-well plates (Ibidi), 20,000 cells per well, and cultured under standard conditions (37 °C, 5% $CO_2$) in minimum essential medium (Sigma Aldrich) supplemented with 10% foetal bovine serum (Gibco) and 2 mM L-lutamine (GlutaMAX, Gibco). After 24 h, cells were fixed by incubation with 4% methanol-free formaldehyde and 0.1% glutaraldehyde in cacodylate buffer (pH 7.4) for 15 min at room temperature, washed three times with PBS and then permeabilised by incubation with a 0.2% solution of saponin in PBS for 15 min. Unspecific binding was blocked by incubating with 10% goat serum and 100 mM glycine in PBS and 0.2% saponin for 30 min at room temperature. Without washing, the samples were incubated with the primary antibody (mouse anti-beta-tubulin: ab131205) diluted 1:200 in PBS containing 2% BSA (bovine serum albumin) and 0.2% saponin overnight at 4 °C. After three washes in PBS, the samples were incubated with the secondary

antibody (goat anti-mouse conjugated to AlexaFluor568) diluted 1:400 in PBS containing 2% BSA and 0.2% saponin for 1 h at room temperature in the dark. Samples were then washed 3 times with PBS and imaged.

# 9 Preparation and Re-organisation of DNA-functionalised Unilamellar Vesicles

## 9.1 Electroformation of de-mixed Giant Vesicles

Giant Unilamellar Vesicles were prepared with electroformation [7, 8, 9]. Briefly, indium tin oxide (ITO) slides underwent a cleaning routine of 15 min sonication cycles of Isopropanol followed by MilliQ water and subsequent drying under a gentle a nitrogen flow. Lipid films were generated on the conductive side of an ITO slide (heated to ~60 °C) by drop casting 45 $\mu$L of lipid mixture (DOPC/DPPC/Chol at a 2:2:1 molar ratio, 4 mg/mL) and gently spreading them with a glass coverslip. The slide was placed in a dry silica dessicator under vacuum for 1 h. Electroformation chambers were assembled using a $\sim$ 1 mm thick polydimethylsiloxane (PDMS) spacer to couple two ITO slides enclosing approximately 400 $\mu$L of filtered sucrose buffer (300 mM). The chambers were connected to a frequency generator with clamps and subjected to a sinusoidal alternating current with voltage amplitude of 2 V with a frequency of 10 Hz for 2 h followed by 1 h at 2 Hz. Finally, vesicles were retrieved gently with a pipette and stored at room temperature in the dark to prevent photobleaching and photooxidation.

## 9.2 DNA nanostructures assembly

The responsive DNA nano-devices were adopted from previous work [10]. DNA oligonucleotides, purchased lyophilised (Integrated DNA Technologies [IDT], Eurogentec, and Biomers) and purified by the supplier with high-performance liquid chromatography (HPLC), were resuspended in Tris-Ethylenediaminetetraacetic acid (EDTA) buffer (1× TE: 10 mM Tris + 1 mM EDTA, pH 8.0) to a final concentration of 100 $\mu$M. DNA nanostructures were subsequently self-assembled with a slow quenching temperature ramp ( 95 °C down to 20 °C at a rate of -0.5 $^\circ C \cdot \text{min}^{-1}$ ) on a thermal cycler (Alpha Cycler 2 PCRMax) in a buffer containing 1× TE +100 mM NaCl. Assembled nanostructures were stored at 4 $^\circ C$ prior to usage.

## 9.3 Vesicle functionalisation with DNA nanostructures

Membrane attachment of DNA nanostructures was done following established functionalisation schemes [10, 11, 12].

Briefly, 9.2 $\mu$L of vesicles were added to a mixture of DNA nanostructures (16.7 $\mu$L) and 57.4 $\mu$L of a correcting buffer, resulting in iso-osmolar conditions containing 1× TE + 100 $\mu$M NaCl + 87 mM Glucose. DNA-GUV mixtures were left overnight under rotation at room temperature and in the dark to avoid photobleaching. During imaging, Fuel/Antifuel strands were added sequentially in iso-osmolar buffers at 10× excess with respect to the anchor modules and the fluorescent cargo to trigger the re-organisation of the vesicles, as shown schematically in Fig. 8.

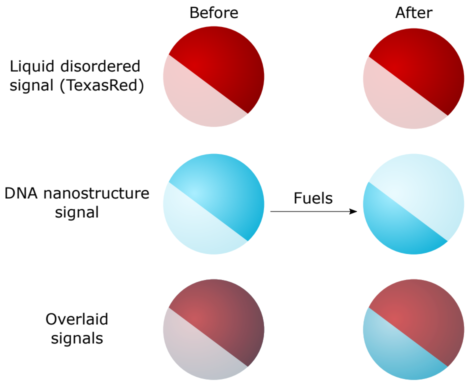


Figure 8: Diagram to show the re-organisation of DNA-functionalised Giant Unilamellar Vesicles. The addition of chemical nucleic-acid signals (fuels) triggers the lateral partitioning of DNA nanostructures (blue) to the liquid-ordered phase. The liquid disordered phase (red) is stained with a fluorescent (TexasRed-DHPE) lipid marker. In the initial configuration, the overlapping DNA and lipid fluorescent signals showcase the preferential affinity of DNA nanostructures for liquid-disordered phases, while cargo transport relocates the fluorescent nanostructures to the liquid-ordered phase.

## 9.4 Sequence of DNA oligonucleotides used

Table 2: **Sequence of DNA oligonucleotides used**

| Strand | Sequence 5' 3' |
|---|---|
| Bbb,chol | /Cholesteryl-TEG/GTTGTGGTGGTGAGTGTG |
| Bb | CATCTCACTACTCAACACCACACTCACCACCACAAC |
| Memf | GTGTTGAGTAGTGAGATG/AlexaFluor488/ |
| Bbb, toc | /Octyl-Tocopherol/GTTGTGGTGGTGAGTGTG |
| Bb, chol | CATCTCACTACTCAACACCACACTCACCACCACAAC/...<br>Cholesterol-TEG/ |
| Cb, chol | /Cholesteryl-TEG/CAATCACACCACAAACACCCAACACAACAAC...<br>AAACC |
| Cbb, chol | GTGTTTGTGGTGTGATTG/Cholesterol-TEG/ |
| Linf,* | GCTCTCTCATCACTAC/AlexaFluor488/ |
| LinF12 | GTGTTGAGTAGTGAGATGATTCGCGTAGTGATGAGAGAGCGTTGT...<br>AGGTTTGTTGTTGTG |
| Fuel1 | GTTGTTGTGTTGGCCTTACTTCACG |
| Antifuel2 | GCGAATCATCTCACTACTCAACACTTCACCTCAAAC |

# References


[1] K. He, X. Zhang, S. Ren, and J. Sun, "Deep residual learning for image recognition," in *Proceedings of the IEEE Computer Society Conference on Computer Vision and Pattern Recognition*, vol. 2016-December. IEEE Computer Society, 12 2016, pp. 770–778.

[2] E. Agustsson and R. Timofte, "NTIRE 2017 Challenge on Single Image Super-Resolution: Dataset and Study," in *IEEE Computer Society Conference on Computer Vision and Pattern Recognition Workshops*, vol. 2017-July. IEEE Computer Society, 8 2017, pp. 1122–1131.

[3] M. A. A. Neil, R. Juškaitis, and T. Wilson, "Method of obtaining optical sectioning by using structured light in a conventional microscope," *Optics Letters*, vol. 22, no. 24, pp. 1905–1907, 1997. [Online]. Available: https://doi.org/10.1364/ol.22.001905

[4] Z. Li, Q. Zhang, S.-W. Chou, Z. Newman, R. Turcotte, R. Natan, Q. Dai, E. Y. Isacoff, and N. Ji, "Fast widefield imaging of neuronal structure and function with optical sectioning in vivo," *Sci. Adv*, vol. 6, 2020. [Online]. Available: https://www.science.org

[5] R. Cao, Y. Chen, W. Liu, D. Zhu, C. Kuang, Y. Xu, and X. Liu, "Inverse matrix based phase estimation algorithm for structured illumination microscopy," *Biomedical Optics Express*, vol. 9, no. 10, p. 5037, 10 2018. [Online]. Available: doi.org/10.1364/BOE.9.005037

[6] E. Ward, "https://github.com/edward-n-ward/ML-OS-SIM," 2023. [Online]. Available: https://github.com/edward-n-ward/ML-OS-SIM

[7] M. I. Angelova, S. Soléau, P. Méléard, F. Faucon, and P. Bothorel, "Preparation of giant vesicles by external AC electric fields. Kinetics and applications," in *Trends in Colloid and Interface Science VI.* Darmstadt: Steinkopff, 1992, pp. 127–131. [Online]. Available: doi.org/10.1007/bfb0116295

[8] M. I. Angelova and D. S. Dimitrov, "Liposome electroformation," *Faraday Discussions of the Chemical Society*, vol. 81, p. 303, 1986. [Online]. Available: doi.org/10.1039/DC9868100303

[9] S. L. Veatch and S. L. Keller, "Separation of Liquid Phases in Giant Vesicles of Ternary Mixtures of Phospholipids and Cholesterol," *Biophysical Journal*, vol. 85, no. 5, pp. 3074–3083, 11 2003.

[10] R. Rubio-Sánchez, S. E. Barker, M. Walczak, P. Cicuta, and L. D. Michele, "A Modular, Dynamic, DNA-Based Platform for Regulating Cargo Distribution and Transport between Lipid Domains," *Nano Letters*, vol. 21, no. 7, pp. 2800–2808, 4 2021. [Online]. Available: https://doi.org/10.1021/acs.nanolett.0c04867

[11] R. Rubio-Sánchez, B. M. Mognetti, P. Cicuta, and L. Di Michele, "DNA-Origami Line-Actants Control Domain Organization and Fission in Synthetic Membranes," *Journal of the American Chemical Society*, vol. 145, no. 20, pp. 11 265–11 275, 5 2023. [Online]. Available: doi.org/10.1021/jacs.3c01493

[12] D. Morzy, R. Rubio-Sánchez, H. Joshi, A. Aksimentiev, L. Di Michele, and U. F. Keyser, "Cations Regulate Membrane Attachment and Functionality of DNA Nanostructures," *Journal of the American Chemical Society*, vol. 143, no. 19, pp. 7358–7367, 5 2021. [Online]. Available: doi.org/10.1021/jacs.1c00166
